# Supplementary material for: Grounded Copilot: How Programmers Interact with Code-Generating Models
Source: arXiv:2206.15000 source file (2022-10-31)
Supplement: Supplementary file 1 [file appendix.tex]

\section{Replication package}
\subsection{Task Programs}
The code for each task is available at \mjsays{Give anonymized link here?}.
% \subsection{Chat Server and Chat Client}
% Our first two tasks, Chat Server and Chat Client share significant code.
% %
% In each language, we first list the shared code, followed by the unique variants.
% %
% \subsubsection{Shared Code}
% \mypara{Python} In Python, the Chat Server and Chat Client each had three files:
% \texttt{crypto.py}, \texttt{server.py}, and \texttt{client.py}.
% %
% Only \texttt{crypto.py} is shared.
% \texttt{crypto.py}:
% \lstset
% { %Formatting for code in appendix
%     language=Python,
%     basicstyle=\ttfamily\footnotesize,
%     numbers=left,
%     stepnumber=1,
%     showstringspaces=false,
%     tabsize=1,
%     breaklines=true,
%     breakatwhitespace=false,
% }
% \lstinputlisting[language=Python]{./replication/copilot-study/chat/py/task1/crypto.py}

% \mypara{Rust} In Rust, the two Chat tasks each have a \texttt{encstream},
% \texttt{crypto\_utils}, \texttt{client}, and
% \texttt{server} subpackage.
% %
% The first two are shared.

% \texttt{encstream}:
% \lstinputlisting[language=Rust]{./replication/copilot-study/chat/rust/task1/encstream/src/encstream.rs}

% \texttt{crypto\_utils}:
% \lstinputlisting[language=Rust]{./replication/copilot-study/chat/rust/task1/crypto_utils/src/crypto_utils.rs}

\subsection{Semi-Structured Interview Questions}
At the end of each session we asked the participant the following questions:
\begin{itemize}
    \item How do you decide which snippets to accept and which to reject?
    \item What could Copilot do differently to help you more?
    \item Did you change your coding style to integrate Copilot in your workflow? If so, how?
    \item How much did you trust Copilot? What should Copilot do to make you trust it more?
    \item What type of programming tasks do you find Copilot most useful for?
    \item What size code suggestions do you like getting from Copilot? Does context matter?
    \item If you like blocks of code as a suggestion, would you prefer to get it
    line-by-line or all-at-once?
    \item How do you like to get your Copilot suggestions? Does context matter?
    \item In what ways do you prefer to invoke Copilot? Does context matter?
\end{itemize}

Afterwards, they could answer any of the following with a
5-point Lickert scale from ``Strongly Disagree''
to ``Strongly Agree''. Participants were encouraged to add a comment if they
had more to say on the question.
\begin{itemize}
    \item I could predict when Copilot would produce useful results
    \item I trust Copilot to give me suggestions that will guide me towards the correct code.
    \item I trust Copilot's suggestions will compile or run without crashing.
    \item In my usages, Copilot should have had enough context to help me.
    \item I trust the quality of Copilot's suggestions more for some languages than others
    \item I appreciate always-on suggestions from Copilot.
    \item I can see myself writing a comment specifically for Copilot's use.
    \item When I know what I need to do, Copilot's suggestions are distracting.
    \item Copilot lowered the overall quality of my code.
    \item Copilot helped me accomplish my task faster than without.
    \item I felt like a more capable programmer with Copilot than I usually feel when working on a new task.
    \item When I was stuck on a task, Copilot's suggestions helped me explore different ways to solve it
    \item When I was stuck on a task, Copilot's suggestions added to my frustration
    \item Copilot helped me come up with the algorithm to solve the task
    \item I found Copilot useful for unfamiliar language syntax
    \item Copilot's suggestions helped me interact with the existing codebase better than without.
    \item Copilot's suggestions helped me use the imported libraries better than without.
    \item Reviewing Copilot's suggestions was mentally taxing.
    \item I felt just the right amount of challenged
    \item My thoughts/activities ran fluidly and smoothly
    \item I didn't notice time passing
    \item I had no difficulty concentrating
    \item My mind was completely clear
    \item I was totally absorbed in what I was doing
    \item The right thoughts/movements occurred of their own accord
    \item I knew what I had to do every step of the way
    \item I felt that I had everything under control
    \item I was completely lost in thought
\end{itemize}
